# Supplementary material for: Probing the Electromagnetic Local Density of States with a Strongly Mixed Electric and Magnetic Dipole Emitter
Source: arXiv:1311.0516 ancillary file (2013-11-03)
Supplement: Supplementary file 1 [file SKaraveli_NiMgO_SuppMat.pdf]

# *Supplemental Material:* Probing the electromagnetic local density of states with a strongly mixed electric and magnetic dipole emitter

Sinan Karaveli,[1,*] Dongfang Li,[1,2] and Rashid Zia[1,2,†]

[1]*School of Engineering, Brown University, Providence, RI 02912, USA*
[2]*Department of Physics, Brown University, Providence, RI 02912, USA*

## Experimental Methods

### Energy-momentum spectroscopy

The energy-momentum spectroscopy technique used in this paper is an updated near-infrared implementation of the method previously described in Ref. [1]. The experimentally acquired s- and p-polarized energy-momentum spectra are shown in Figs. S1(a) and S1(b). We fit the p-polarized momentum cross sections at each wavelength to theoretical cross sections calculated for isotropic ED and MD emitters located at the center of the 37 nm MgO thin film (n=1.66). As described in detail in Ref. [1], this allows us to decompose the observed energy spectrum, shown in Fig. S1(c), into ED and MD contributions. Note that the narrow features seen near 1.4 $\mu$m are minor artefacts due to water absorption lines. The differing signal intensities and room humidity conditions between the Ni:MgO fluorescence and calibration lamp measurements resulted in the introduction of these small oscillations with the spectral calibration procedure. Figures S1(d) and S1(e) show the theoretical energy-momentum spectra for both s- and p-polarization, which corresponds very well with the experimental data. The momentum cross sections shown in Fig. S1(g) show that the theoretical fits match the experimental results very well for both polarizations. (The improved quality of these fits as compared to those in Ref. [1, 2] results from the enhanced imaging resolution provided by the Schmidt-Czerny-Turner spectrograph and the use of a longer focal length Bertrand lens.)

### Lifetime measurements

Due to their high inherent noise, InGaAs SPADs are not operated in free running mode but are instead periodically gated by applying the bias voltage only for a short duration (gate width) at a high frequency (gate frequency). Upon a trigger event, i.e. detection of a photon or dark count, the detector is immediately turned off for a duration $T_{off}$ to minimize any after-pulsing related counts. In order to prevent any distortion of lifetime measurements due to photon-pile up and detector saturation effects, the time-correlated single photon counting (TCSPC) measurements are performed in a low fluence regime where the photon detection rate is less than 10% of the laser repetition rate, i.e. less than 10 detected photons for 100 laser pulses [3]. This is especially important in SPADs as higher photon count rates increase the probability of a second photon arrival during the SPAD off-time during which it cannot be registered. This can skew the photon detection histogram and result in the so-called "photon pile-up" effect.

The long (>1ms) lifetime of $Ni^{2+}$ requires a low laser repetition rate in order to resolve the slow decay of the emitters. This makes the conventional approach of TCSPC measurements with a photon count rate <10% of the laser repetition rate impractical for such long lifetime emitters. An alternative approach is to set the SPAD settings such that the detector is gated at a period ($T_{period}$) that is longer than the hold-off time ($T_{off}$) and adjust the gate-width ($T_{GW}$) to get a photon count rate per gate period that is 1-5%. This allows for uniform sampling of the time decay while preventing any histogram distortion due to saturation effects. In addition, because the SPAD can only detect one photon per gate period, we use the gate frequency trigger output of the SPAD controller as the external time-binning clock ($T_{bin}$) of the multichannel analyzer. The specific settings used for lifetime measurements in this study were as follows: $T_{GW}$ = 50 ns, $T_{off}$ = 12 $\mu$s, $T_{period}$ = $T_{bin}$ = 12.5 $\mu$s.

*Present address: Research Laboratory of Electronics, Massachusetts Institute of Technology, Cambridge, MA 02139, USA
†Electronic address: Rashid_Zia@brown.edu

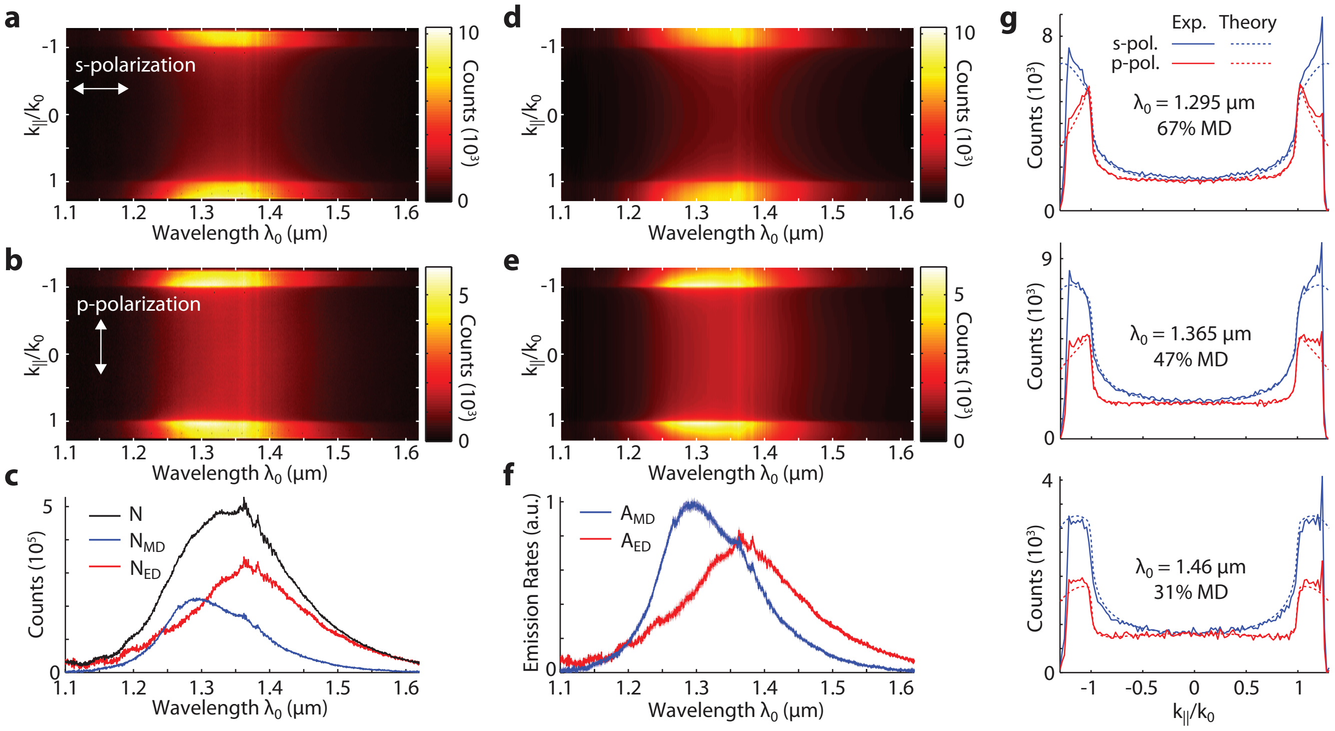


FIG. S1: Quantifying the broad $^3T_2 \rightarrow {}^3A_2$ emission sideband in $Ni^{2+}$:MgO by energy-momentum spectroscopy. (a,b) Experimental energy-momentum spectra acquired for s- and p-polarization, respectively. (c) Integrated energy spectrum of the total observed emission (N, black line) decomposed into the contributions from ED ($N_{ED}$, red line) and MD ($N_{MD}$, blue line) transitions. (d,e) Theoretical energy-momentum spectra for s- and p-polarization, respectively, produced using fits to Equation 1 in Ref. [1]. (f) Spectrally-resolved emission rates, $A_{ED}$ (solid red line) and $A_{MD}$ (solid blue line), deduced from fitting analysis together with their 95% confidence intervals (shaded regions). (g) Momentum cross sections showing that experimental data (solid lines) from strongly mixed transitions can be readily resolved by theoretical fits (dashed lines).

## Analysis of Lifetime Results

### LDOS calculations

For the three layer planar structure considered in the manuscript, the normalized electric and magnetic LDOS expressions are [4]:

$$\tilde{\rho}^E(\lambda, d) = \frac{1}{2}\,\mathrm{Im}\Big[\int_0^\infty \Big(\frac{(1+R^s_{12})(1+R^s_{13})}{1-R^s_{12}R^s_{13}} + \frac{(1+R^p_{12})(1+R^p_{13}) - 2u^2(R^p_{12}+R^p_{13})}{1-R^p_{12}R^p_{13}}\Big)\frac{udu}{l_1}\Big], \tag{S1}$$

$$\tilde{\rho}^M(\lambda, d) = \frac{1}{2}\,\mathrm{Im}\Big[\int_0^\infty \Big(\frac{(1-R^p_{12})(1-R^p_{13})}{1-R^p_{12}R^p_{13}} + \frac{(1-R^s_{12})(1-R^s_{13}) + 2u^2(R^s_{12}+R^s_{13})}{1-R^s_{12}R^s_{13}}\Big)\frac{udu}{l_1}\Big]. \tag{S2}$$

where $R^{s,p}_{ij} = r^{s,p}_{ij}\exp(-2kl_i s_{ij})$ represents the reflected electric field from the $i,j$ interface at the emitters location. $r^s_{i,j} = (l_i - l_j)/(l_i + l_j)$ and $r^p_{i,j} = (\varepsilon_i l_j - \varepsilon_j l_i)/(\varepsilon_i l_j + \varepsilon_j l_i)$ are the reflection coefficients for s- and p-polarization, and $s_{ij}$ is the distance of the emitter from the $i,j$ interface. The subscript index 1 designates the central layer in which the emitter is embedded (MgO, $n_1$=1.66), while indices 2 and 3 represent the bottom (quartz) and top layers (air or metal), respectively. The emitter distance from the quartz substrate ($n_2$=1.44) is fixed at $s_{12}$=18.5 nm, and the emitter distance from the gold or air is varied with the MgO spacer thickness such that $s_{13}$=$d$. For the metal coated cases, the gold refractive index is calculated using the Brendel-Bormann model [5]. $u = k_\parallel/k$ and $l_j = -i\sqrt{{n_j}^2/{n_1}^2 - u^2}$ are the parallel and perpendicular components of the wavevector normalized to the emitter layer wavenumber, $k = (2\pi/\lambda)n_1$. For the lossless case of top air layer ($n_3 = 1$), the above expressions include singularities associated with the waveguide modes which can be difficult to treat numerically. For practical

cases, this problem can addressed by including a small, realistic amount of loss either in the material refractive indices themselves or at each interface to account for scattering losses. We numerically calculated a variety of cases with small ($\kappa = 10^{-3} - 10^{-4}$) losses added into the MgO or air layers, and losses to reflections on each dielectric interface. All cases produce very similar results. Those shown in this manuscript are specifically for the case of a 0.5% reflection loss added to the air-MgO interface.

**Decay rate calculations and fits to lifetime variations**

The lifetime of the emitters at different distances $d$ from the air or gold interfaces will be modified compared to their lifetime in the bulk medium, $\tau_0$, according to the following equation [4]:

$$\tau(d) = \tau_0(1 - q(1 - \tilde{\Gamma}(d)))^{-1} \tag{S3}$$

where $q$ is the quantum efficiency and $\tilde{\Gamma}(d) \equiv \Gamma(d)/\Gamma_0$ is the total radiative decay rate normalized to the bulk medium case. In the literature, $\tilde{\Gamma}(d)$ is usually taken as the isotropic average of the normalized radiative decay rate for an ED emitter and calculated at the spectral peak for a single wavelength [4]. As the emission of $Ni^{2+}$:MgO is very broad and the ED and MD transitions have slightly different spectral distributions, one needs to take into account the effect of LDOS variations at different wavelengths. To this end, we have used the spectrally-resolved intrinsic ED and MD emission rates obtained by energy-momentum spectroscopy and calculated the $\tilde{\Gamma}^{Iso}_{MD}(d)$ and $\tilde{\Gamma}^{Iso}_{ED}(d)$ as follows:

$$\tilde{\Gamma}^{Iso}_{MD}(d) = \int \tilde{A}_{MD}(\lambda)\tilde{\rho}^{M}(\lambda, d)d\lambda \tag{S4}$$

$$\tilde{\Gamma}^{Iso}_{ED}(d) = \int \tilde{A}_{ED}(\lambda)\tilde{\rho}^{E}(\lambda, d)d\lambda \tag{S5}$$

where $\tilde{A}_{MD}(\lambda)$ and $\tilde{A}_{ED}(\lambda)$ are the spectrally-resolved MD and ED emission rates normalized such that $\int \tilde{A}_{MD,ED}(\lambda)d\lambda = 1$.

The experimentally observed lifetime variations were then fit to Eq. S3 using $\tilde{\Gamma}(d) = a_{MD}\tilde{\Gamma}^{Iso}_{MD}(d) + (1 - a_{MD})\tilde{\Gamma}^{Iso}_{ED}(d)$ where $a_{MD}$ is the MD percentage of total emission that we use as a fit variable together with $\tau_0$. The resulting fits are shown as solid purple lines in Fig. 4 of the main text and here in Fig. S2. As a comparison, we have also performed similar fits assuming that all the observed emission originates from purely ED or MD emitters. Specifically, we have used Eq. S3 with $\tau_0$ and $q$ as the free fit parameters and $\tilde{\Gamma}^{Iso}_{MD,ED}(d) = \int \tilde{A}(\lambda)\tilde{\rho}^{M,E}(\lambda, d)d\lambda$ where $\tilde{A}(\lambda)$ is the normalized emission spectrum of $Ni^{2+}$. The resulting fits, shown as the red and blue curves in Fig. S2, clearly do not correspond to the experimental results. Note also that the individual fits for either ED or MD only emitters yield markedly different quantum yields for the two different experimental cases, i.e. the metal and air coated data.

Finally, we also directly compare the experimental lifetime results to theoretical calculations without any fit parameters. To this end, we use $\tau_0 = 2.8$ ms which we obtained by measuring the lifetime of $Ni^{2+}$ ions in a bulk single-crystal MgO, approximate the quantum yield by $q = \tau_0/3.6$ ms as described in the main text, and use $a_{MD} = 0.504$ as obtained from the energy-momentum characterization ($a_{MD} = \int A_{MD}(\lambda)d\lambda / \int (A_{MD}(\lambda) + A_{ED}(\lambda))d\lambda$). The results are shown in Fig. S3.

---


[1] T. H. Taminiau, S. Karaveli, N. F. van Hulst, and R. Zia, Nat. Commun. **3**, 979 (2012).

[2] S. Karaveli, S. Wang, G. Xiao, and R. Zia, ACS Nano **7**, 7165 (2013), ISSN 1936-0851.

[3] W. Becker, *Advanced Time-Correlated Single Photon Counting Techniques*, Springer Series in Chemical Physics Series (Springer Berlin Heidelberg, 2005).

[4] R. R. Chance, A. Prock, and R. Silbey, Adv. Chem. Phys. **37**, 1 (1978).

[5] A. D. Rakic, A. B. Djurišic, J. M. Elazar, and M. L. Majewski, Appl. Opt. **37**, 5271 (1998).

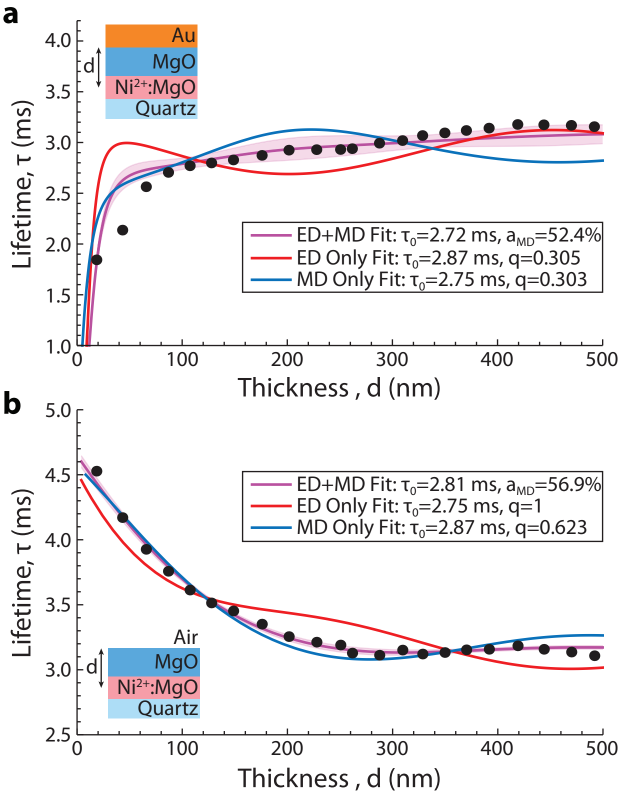


FIG. S2: Lifetime data acquired for $^3T_2$ state of $Ni^{2+}$:MgO near (a) a gold mirror and (b) an air interface together with fits to the purely electric LDOS (red line), purely magnetic LDOS (blue line), and mixed electromagnetic LDOS (purple line). The legends for each subpanel include the obtained lifetime ($\tau_0$) and quantum yield (q) for each fit. Shaded purple region shows the 95% confidence interval for the mixed electromagnetic fit.

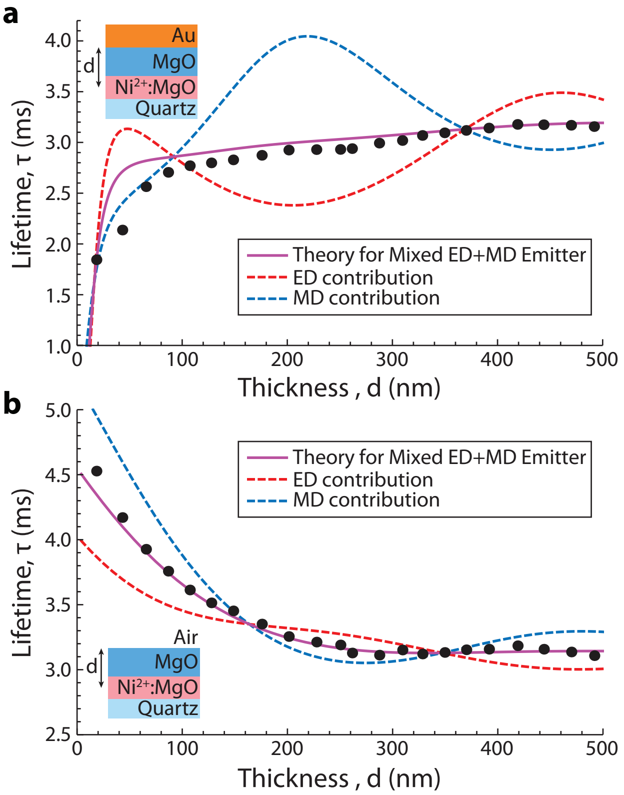


FIG. S3: Comparison of lifetime data to theoretical calculations obtained for strongly mixed ED-MD emitters without any fit parameters (solid purple lines) by directly using the ED and MD percentages from the energy-momentum spectroscopy analysis. For completeness, we also plot the electric (dashed red) and magnetic (dashed blue) contributions to the electromagnetic LDOS for this strongly mixed ED-MD case, i.e. the variations expected for ED and MD transitions which are then averaged according to the energy-momentum spectroscopy percentages to obtain the purple curve.
